# Supplementary material for: Low-count Time Series Anomaly Detection
Source: arXiv:2308.12925 source file (2023-08-24)
Supplement: Supplementary file 1 [file appendix.tex]

\section{Additional Plots}

\begin{figure}[htp]
\begin{minipage}[b]{.48\linewidth}
  \centering
  \centerline{\includegraphics[width=4.0cm]{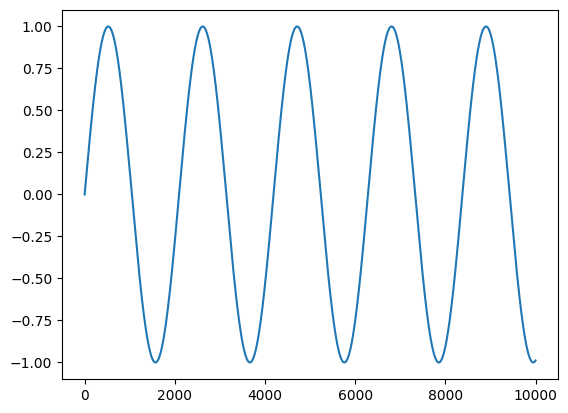}}
%  \vspace{1.5cm}
  \centerline{(a) Seasonal Time Series}\medskip
\end{minipage}
\hfill
\begin{minipage}[b]{0.48\linewidth}
  \centering
  \centerline{\includegraphics[width=4.0cm]{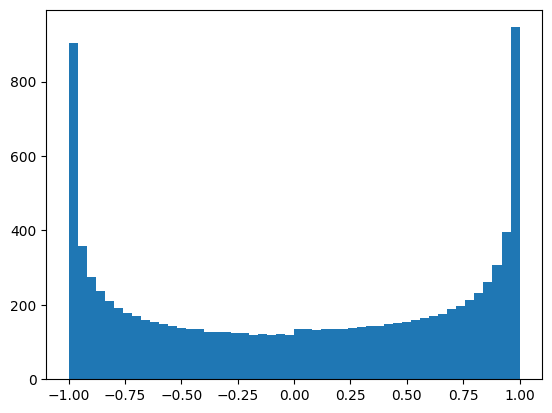}}
%  \vspace{1.5cm}
  \centerline{(b) Distribution}\medskip
\end{minipage}
\caption{Distribution of a seasonal time series.}
\label{fig:seasonal_distribution}
\end{figure}

\begin{figure}[htp]
  \centering
  \centerline{\includegraphics[width=8.5cm]{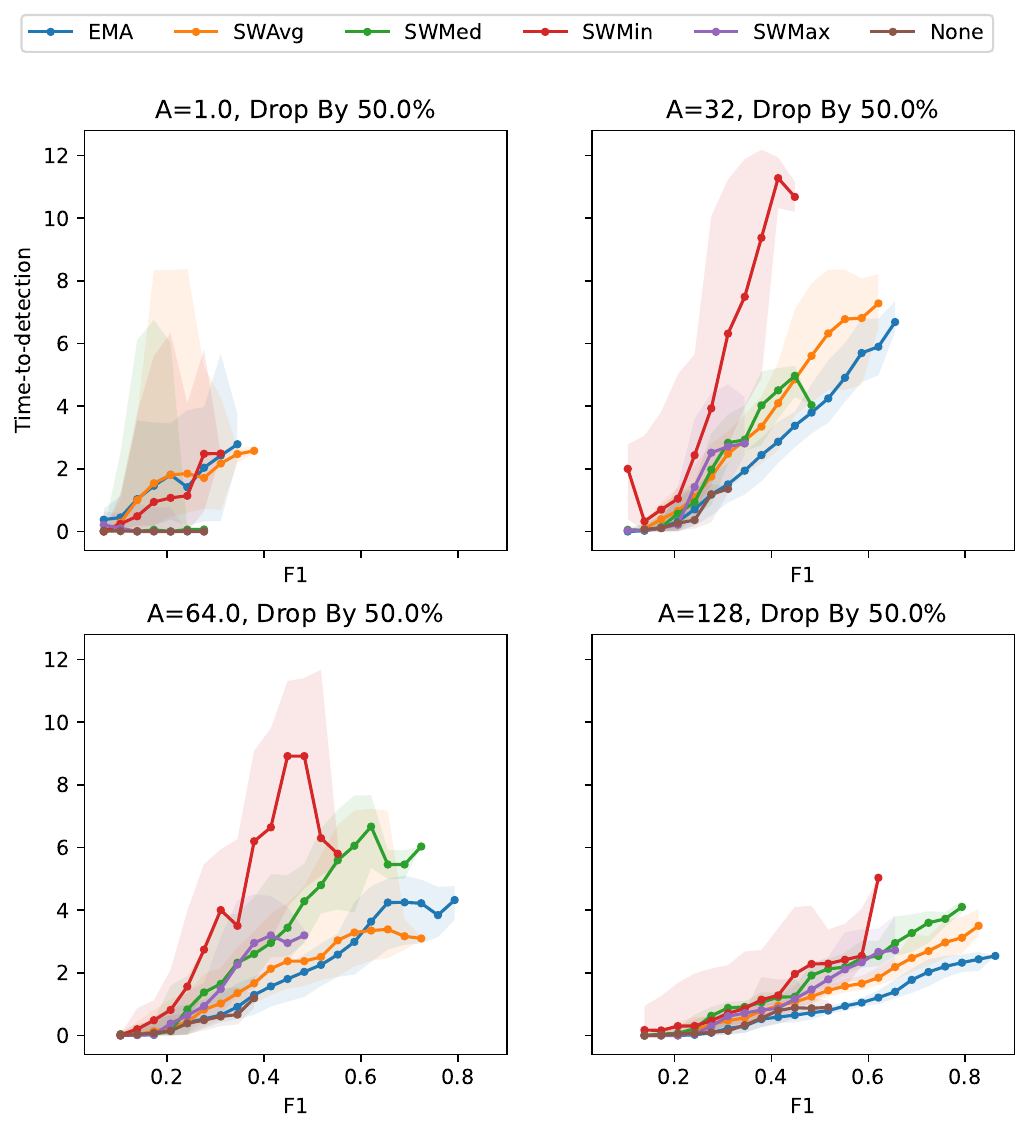}}
%  \vspace{2.0cm}
\caption{How the F1 and time-to-detection changes with different smoothing functions.}
\label{fig:time_to-detection_full}
\end{figure}

\section{M5 Data Pre-processing}
\label{appendix:m5_preprocessing}
To categorise the M5 dataset into count level groups, we predefined the mean of each group to  and it is worth noting that the time series with the lowest count level of this dataset cannot cover intermittent cases. Therefore, we randomly zeroed out values with a binomial distribution over a random selection of time series to widen the generalisation of the experiment. T
